# Supplementary material for: Observation of $Z$ production in proton-lead collisions at LHCb
Source: arXiv:1406.2885 source file (2014-10-14)
Supplement: Supplementary file 1 [file supplementary.tex]

\section*{Supplementary material for LHCb-PAPER-2014-022
\label{sec:Supplementary}}

\begin{figure}[htbp]
\begin{center}
\includegraphics[width=0.7\textwidth]{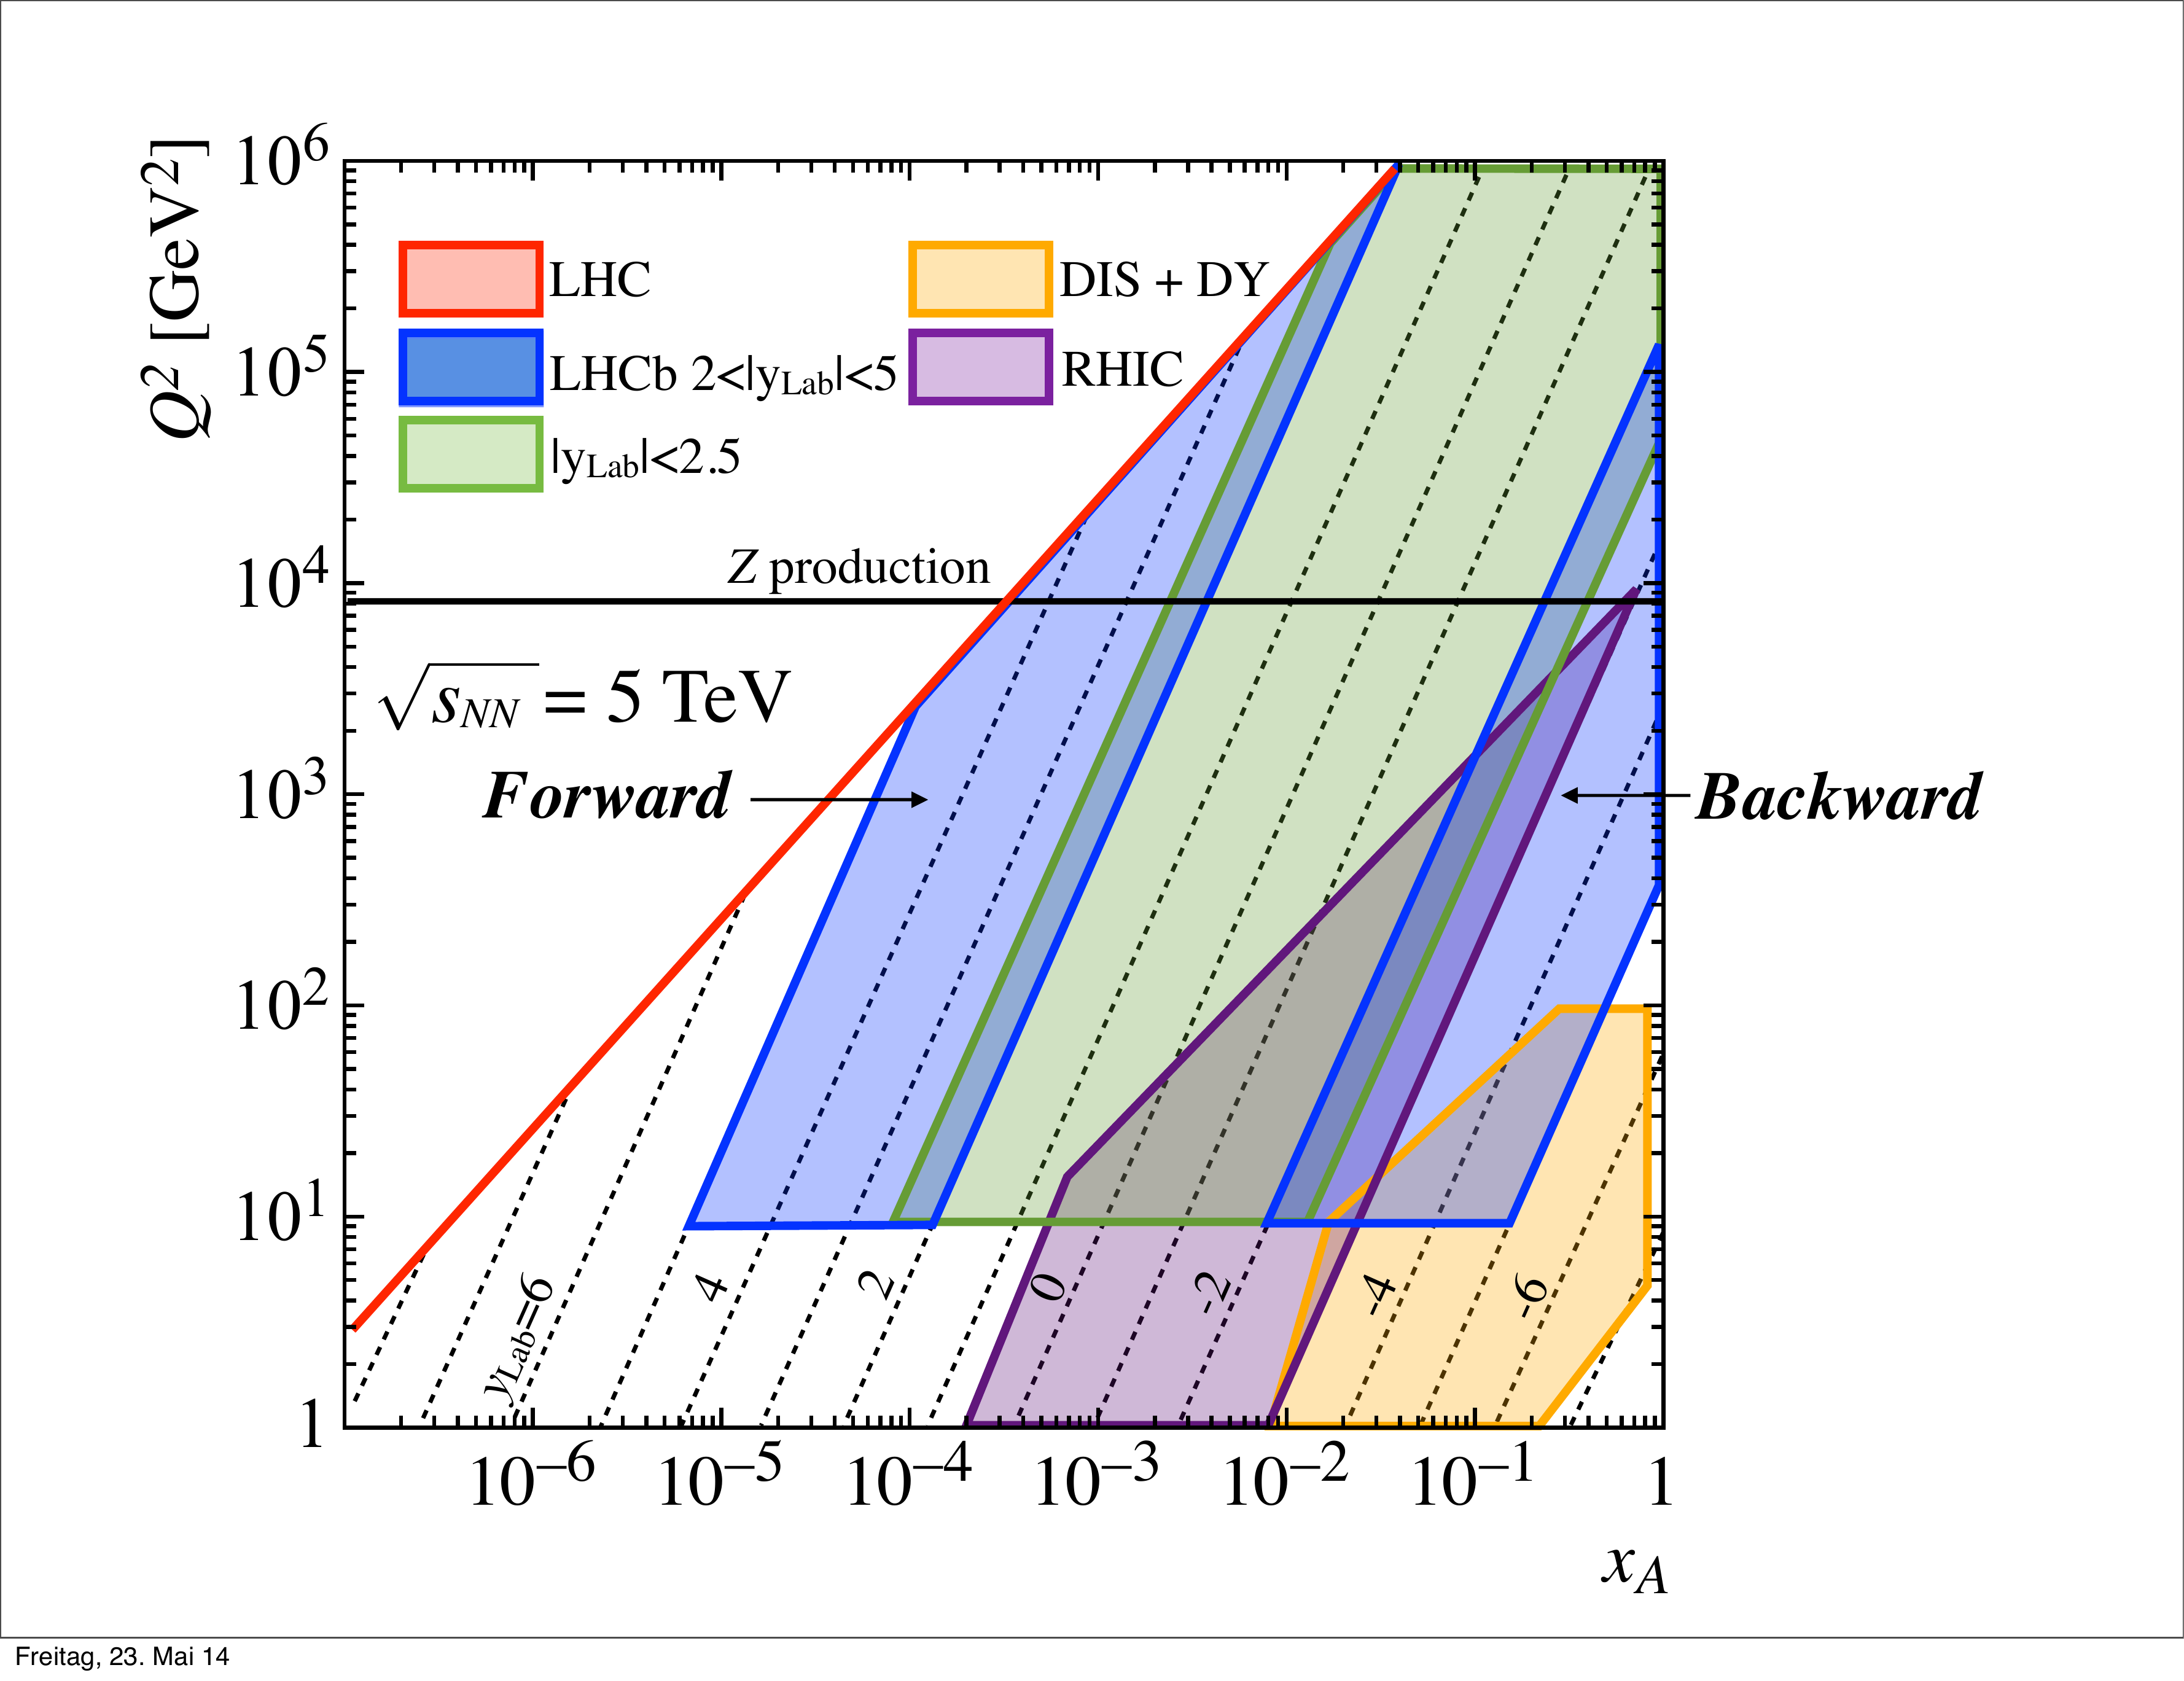}
\caption[$x_A$-$Q^2$-space accessible to different experiments]{Regions in $x_A$-$Q^2$ that LHC, RHIC (purple area) or fixed target experiments (DIS + DY; yellow area) are sensitive to. The centre-of-mass energy per proton-nucleon pair for LHC is $\sqrt{s_{pN}}=5\tev$. The red line shows the kinematic boundary for this particular centre-of-mass energy. The blue area shows the sensitive region for LHCb for energy scales $Q^2>10~\text{GeV$^2$}$. The black horizontal line corresponds to the mass of the \Z boson indicating that LHCb is sensitive down to $x_A \approx 2\cdot 10^{-4}$ for measurements of the \Z production. The green area shows the phase space corresponding approximately to the ATLAS and CMS detector and the central part of the ALICE detector. Process dependent phase spaces of these experiments can be seen in Ref.~\cite{Salgado:2012}. The regions for RHIC and fixed target experiments have been also taken from Ref.~\cite{Salgado:2012}. The corresponding rapidity in the laboratory frame is shown by the dashed lines and indicated by the numbers in the plot. For the rapidity, $y$, in the centre-of-mass frame there is a shift of $y_\text{Lab}-y=\Delta y=+0.47$ with respect to the rapidity, $y_\text{Lab}$, in the laboratory frame.}
\label{fig:xQ2_pA}
\end{center}
\end{figure}

\begin{figure}[htbp]
\begin{center}
\begin{minipage}[t]{0.49\textwidth}
\begin{overpic}[width=\textwidth,scale=.25,tics=20]{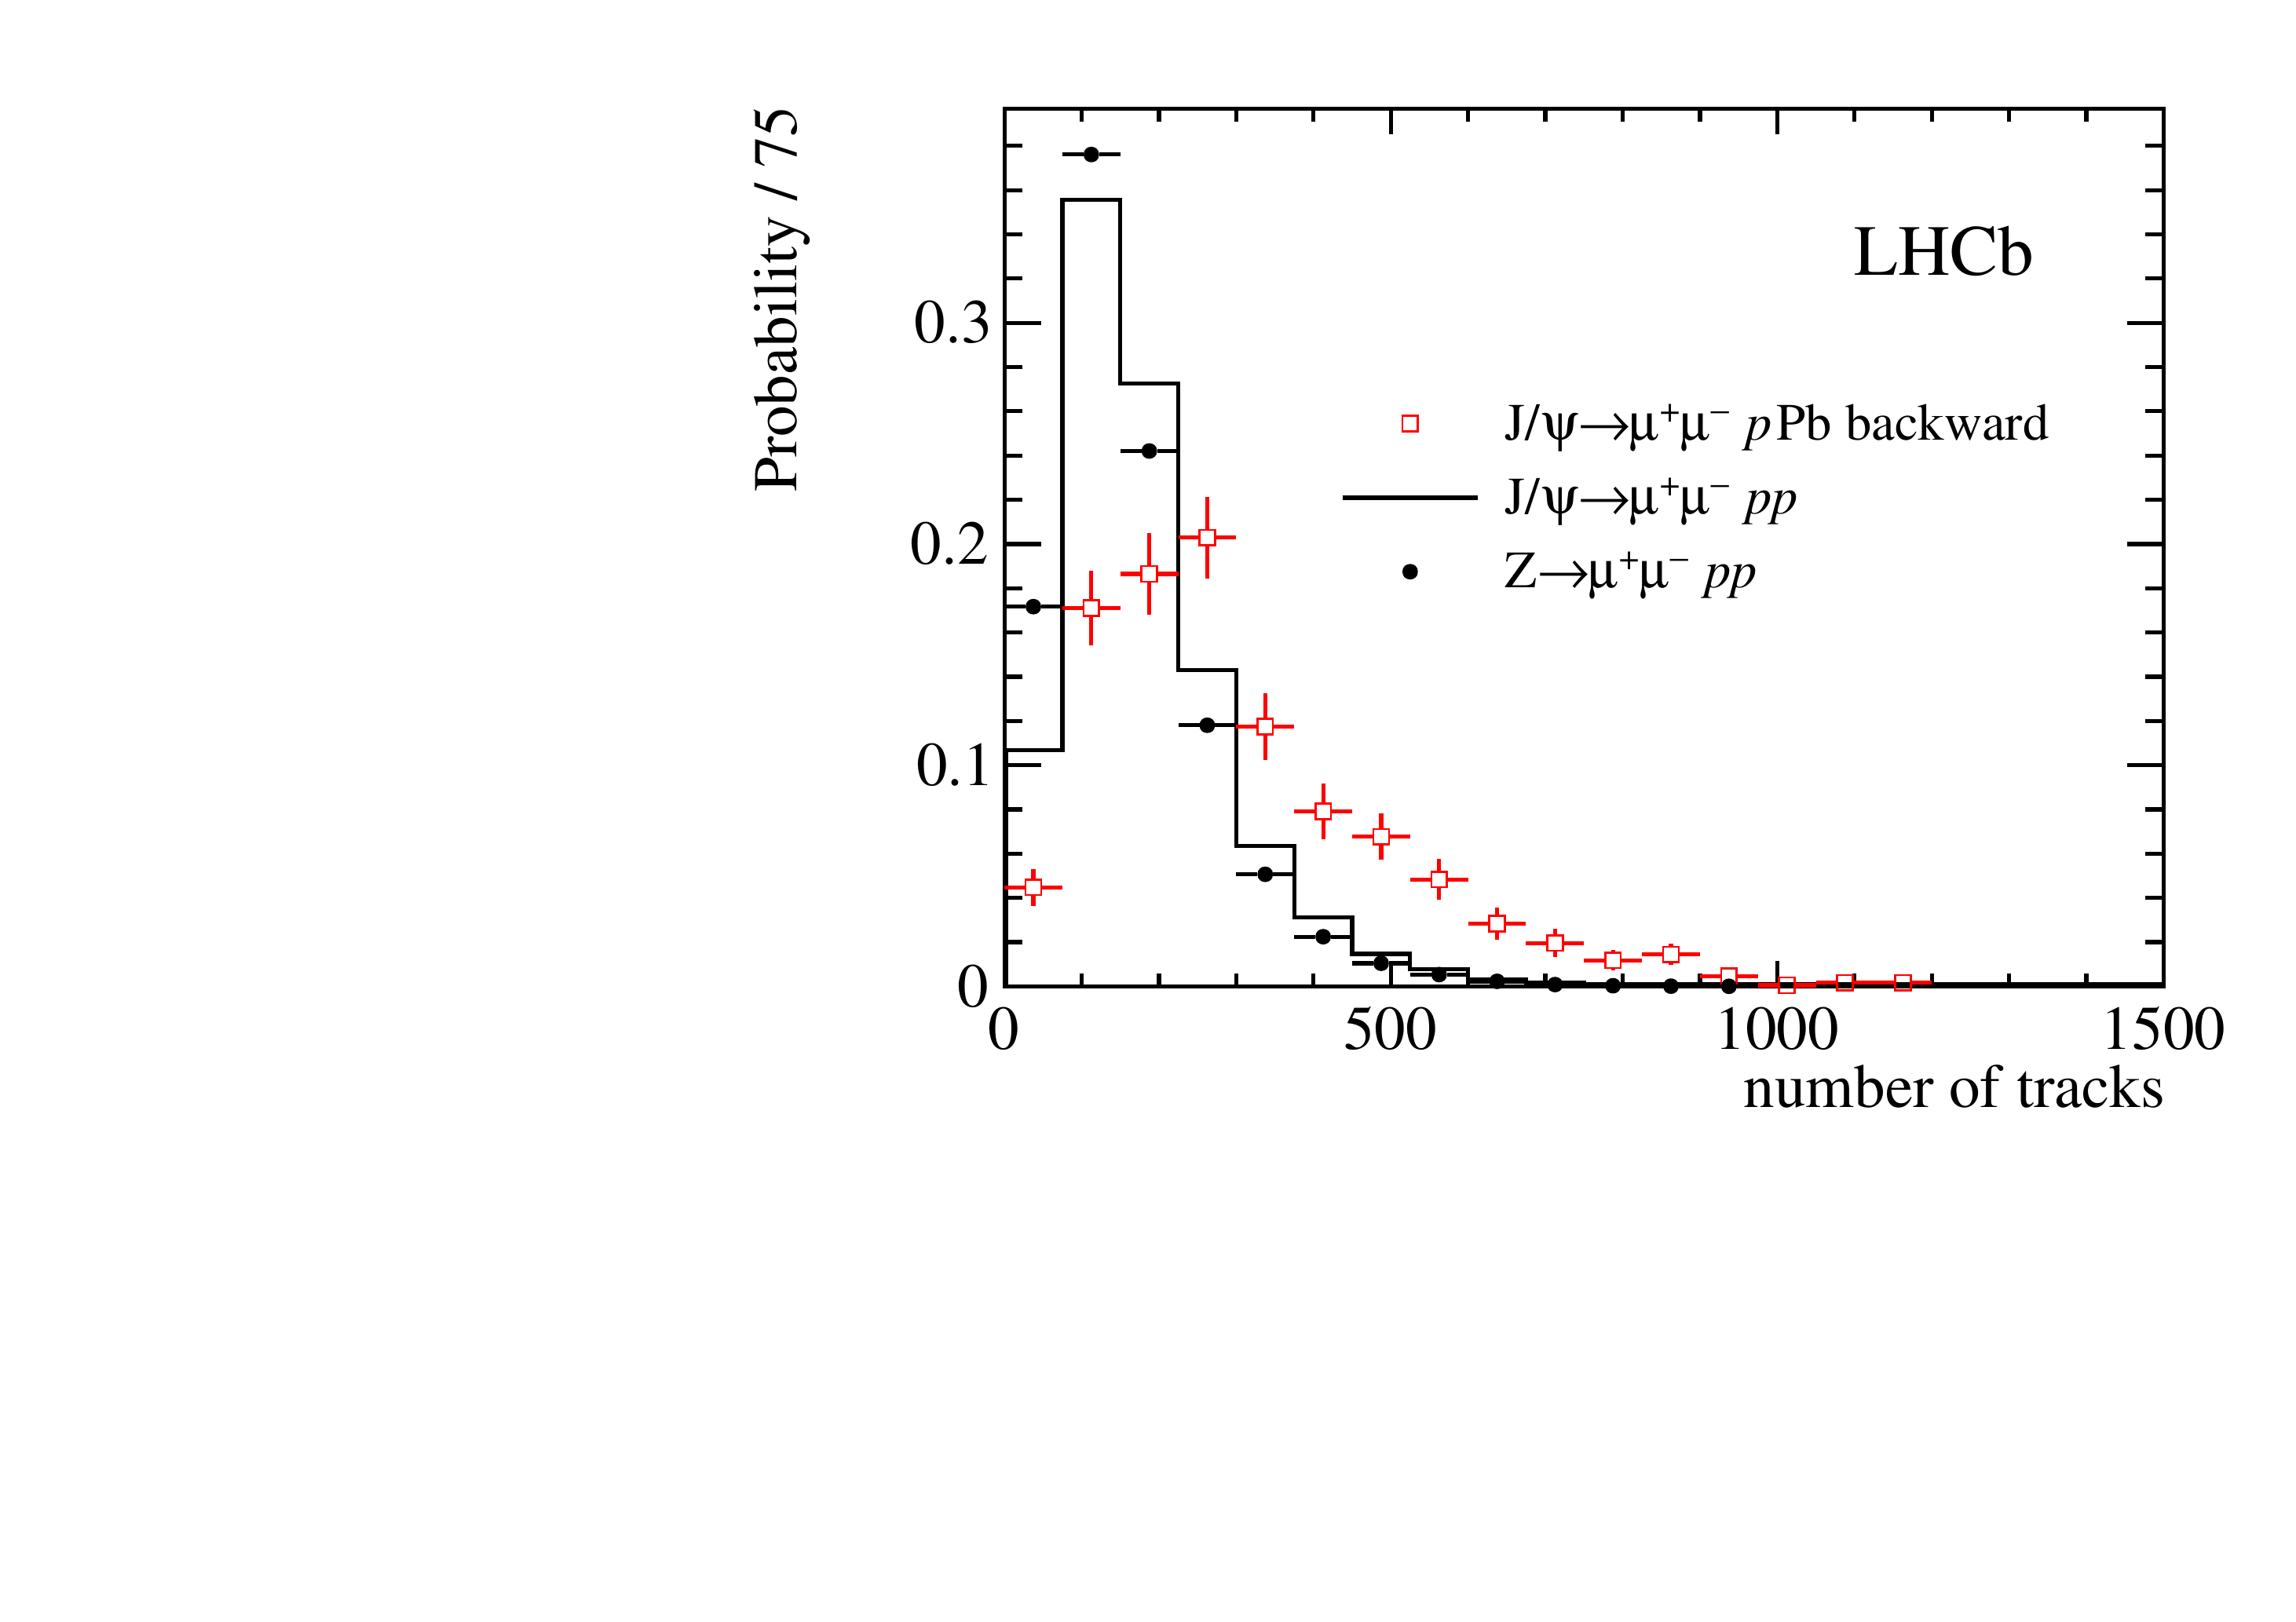}
\put(80,30){(a)}
\end{overpic}
\end{minipage}
\begin{minipage}[t]{0.49\textwidth}
\begin{overpic}[width=\textwidth,scale=.25,tics=20]{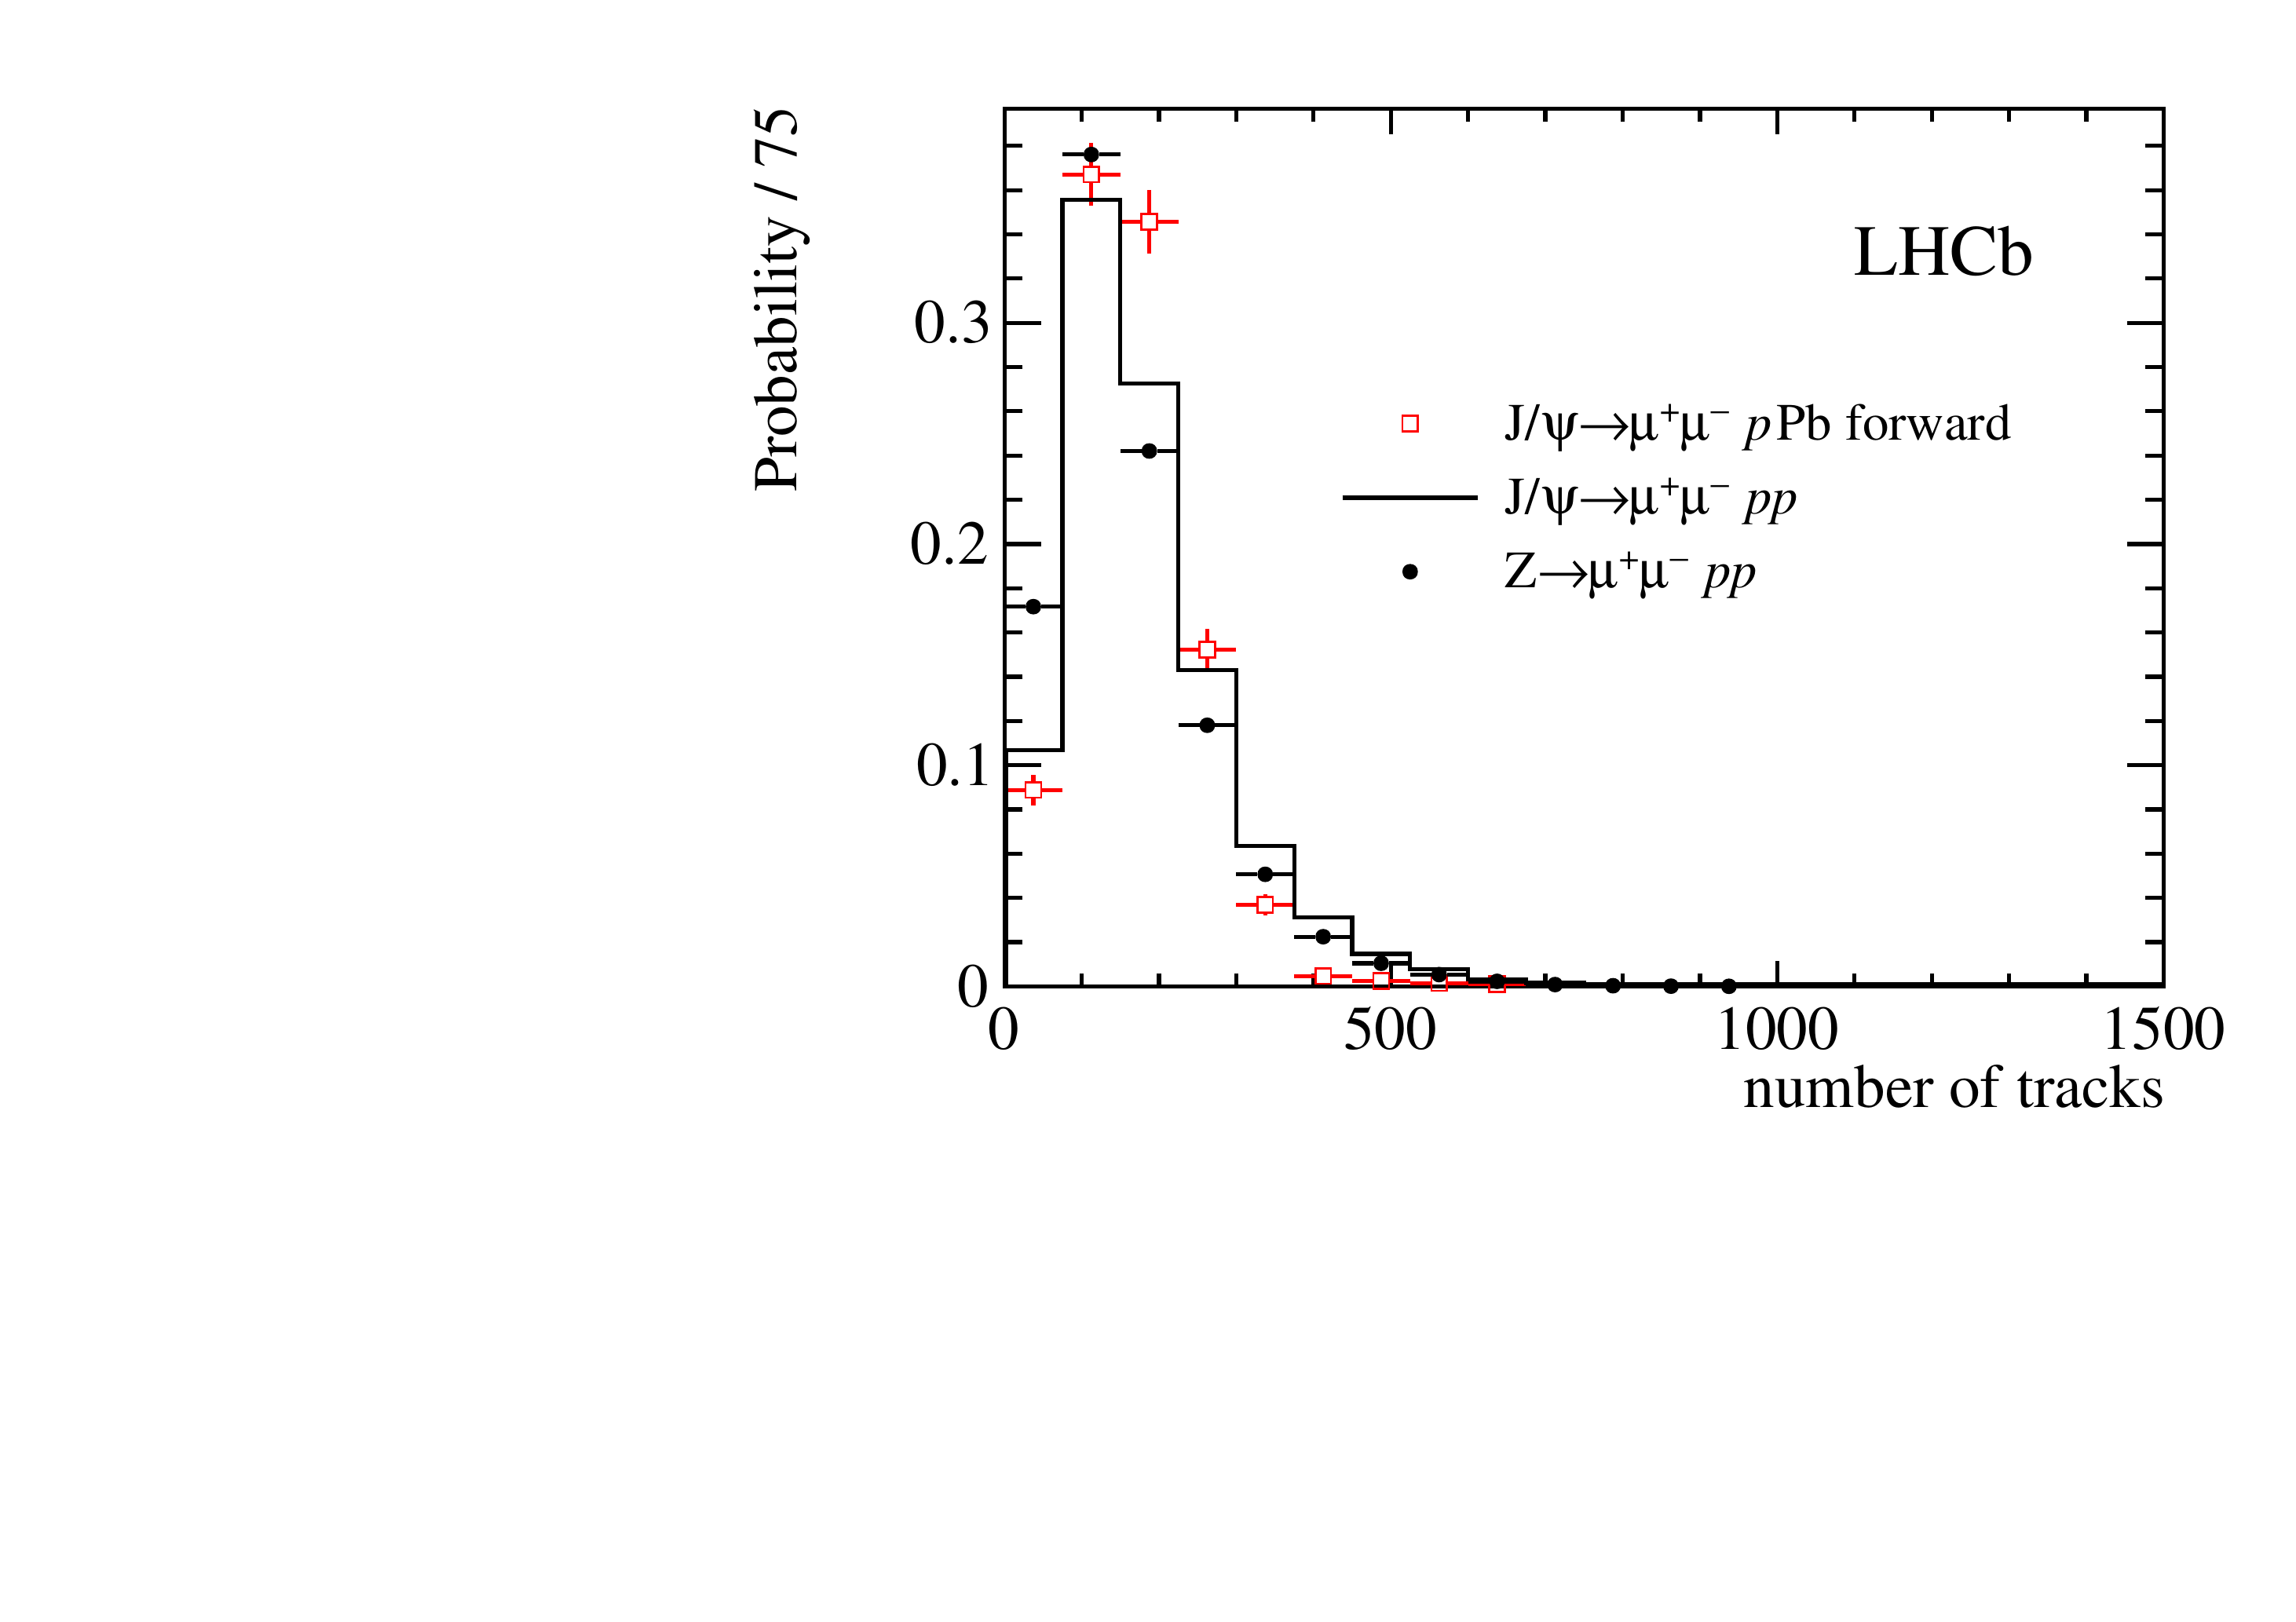}
\put(80,30){(b)}
\end{overpic}
\end{minipage}
\caption[Track multiplicity distribution]{The track multiplicity distributions of events containing \jpsi candidates in (a) the backward and in (b) the forward direction are shown by the red data points. For comparison the distributions for events with \jpsi (black solid line) as well as \Z (black dots) candidates in $pp$ collisions at $\sqrt{s}=8\tev$ recorded in 2012 are displayed.\\
The similarity of the distributions in the forward sample between $pp$ and $p$Pb collisions is rather accidental as the two effects of a smaller pile-up in $p$Pb collisions and of collisions of the proton with a lead nucleus cancel each other out. The higher track multiplicity in the backward sample is caused by the lead nucleus propagating toward the detector.}
\label{fig:multi}
\end{center}
\end{figure}

\begin{figure}[htbp]
\begin{center}
\begin{minipage}[t]{0.7\textwidth}
\begin{overpic}[width=\textwidth,scale=.25,tics=20]{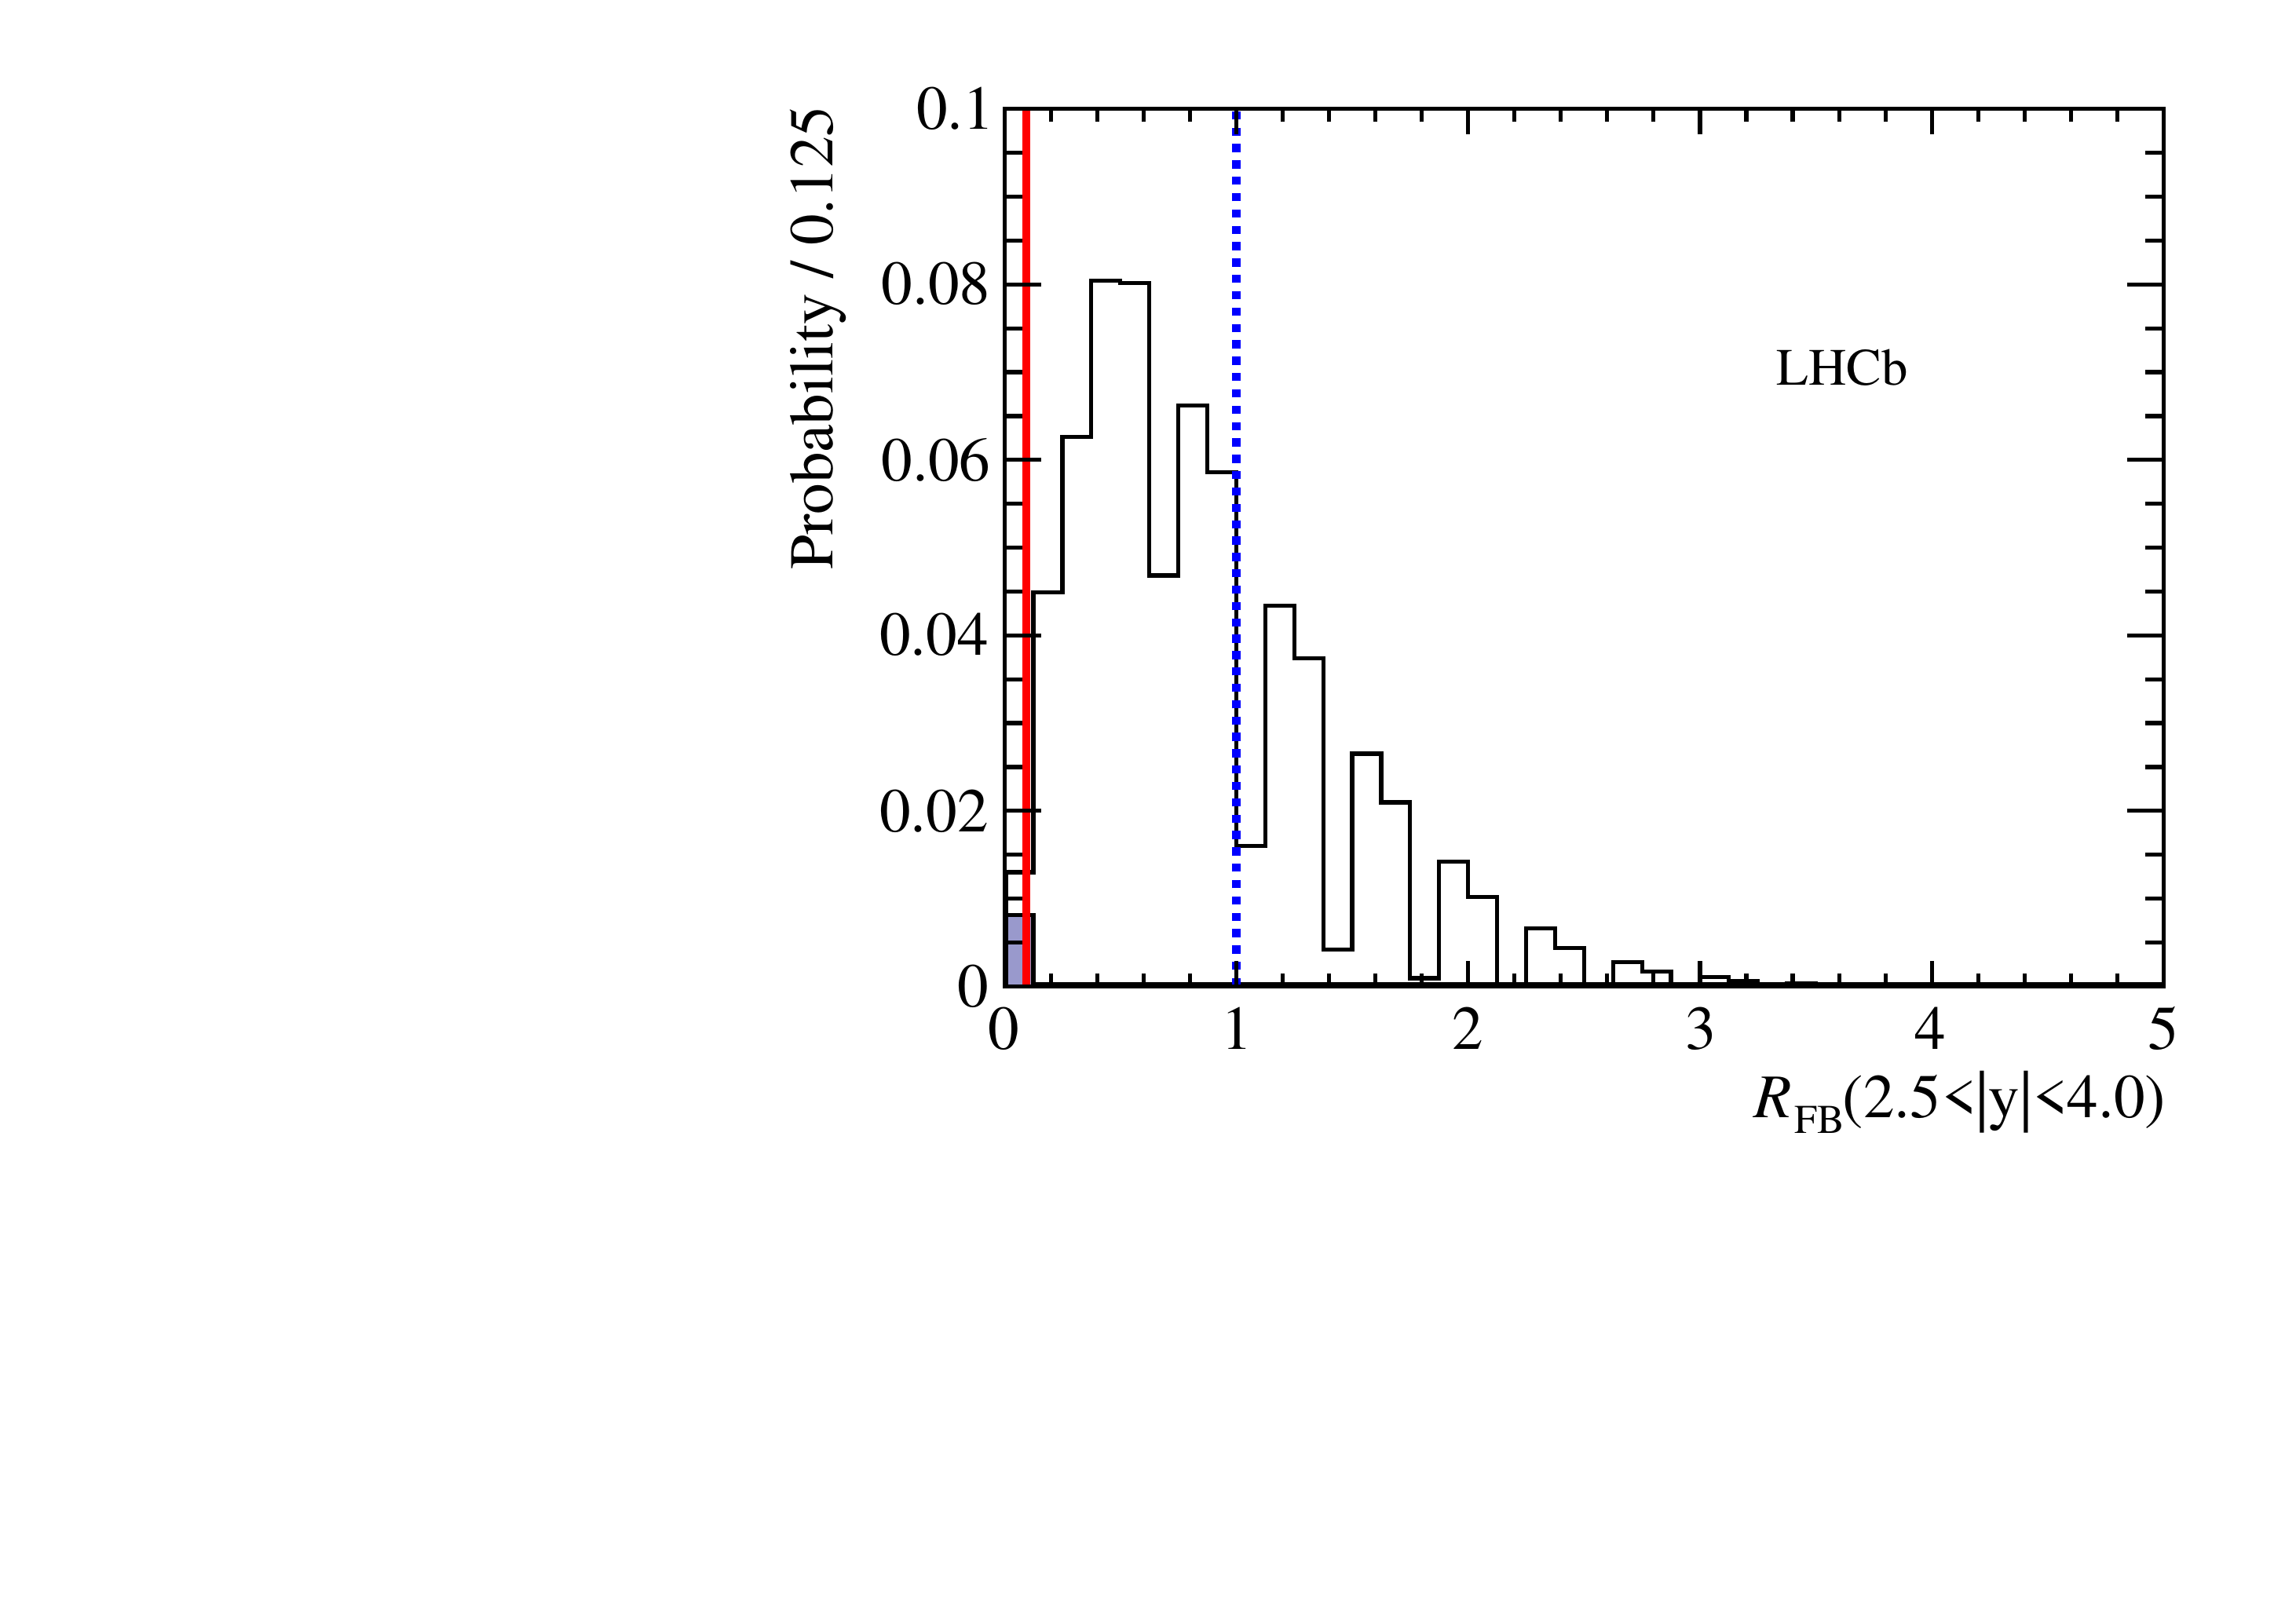}
\end{overpic}
\end{minipage}
\caption[Track multiplicity distribution]{Distribution of $R_\text{FB}(2.5<|y|<4.0)$ for a true value of 1.0 from Toy Monte Carlo. The solid red line shows the central value and the dashed blue one $R_\text{FB}(2.5<|y|<4.0)=1.0$ The filled part of the histogram shows the region below the observed value, it corresponds to a $p$-value of 0.012. The discrete behaviour of the plot originates from the fact that the ratio is built from integers.}
\label{fig:R_FB_dist}
\end{center}
\end{figure}
